# Supplementary material for: Joint learning of a network of linear dynamical systems via total variation penalization
Source: arXiv:2511.18737 source file (2026-07-05)
Supplement: Supplementary file 1 [file appendix_additional_exps.tex]

%-----------------------------------
% Additional experimental results
%
\section{Additional experimental results} \label{appsec:additional_exps}
\subsection{Implementation details and defaults}
All experiments are implemented in \textsf{R} using \texttt{genlasso}, \texttt{igraph}, \texttt{Matrix}, \texttt{ggplot2}, \texttt{dplyr}, and \texttt{tidyr}.
The design matrices use Kronecker products and block-diagonal concatenation; both $Q$ and $y$ are scaled by $1/\sqrt{m}$.
We use the validation split to select $\lambda$ and report all errors on the held-out test split.
Unless otherwise noted:
\begin{itemize}
  \item \textbf{State dimension:} $d=2$;
  \item \textbf{Splits:} $T_{\text{val}}=4$, $T_{\text{test}}=8$;
  \item \textbf{Regularization path:} up to 200 steps;
  \item \textbf{Replicates:} $n_{\text{rep}}=5$ for curves ($T$ and $m$ sweeps), and $n_{\text{rep}}=3$--$4$ for path plots;
  \item \textbf{Grids:} typical $(n_x,n_y)=(20,15)$ for $T$-sweeps; $(6,6)$--$(12,12)$ for $m$-sweeps;
  \item \textbf{Star:} $m\in\{10,20,50,100\}$, $\Delta\in[0.05,0.3]$.
\end{itemize}
\hemant{The above text can be polished. For instance, some of the notation has not been explained. Also its not clear why the star graph appears here since the experiments seem to be only for real data where the k-NN graph was used in the main text.}

\subsection{Qualitative summary}
At small $T$, TV substantially outperforms OLS\textsubscript{ind} (and OLS\textsubscript{pooled} on heterogeneous fields) by borrowing statistical strength across nodes; as $T$ grows, TV approaches OLS\textsubscript{ind}. TV benefits from increasing $m$ on both graphs. On the grid, increasing the spatial frequency $\omega$ (less piecewise-constant fields) diminishes TV's advantage; on the star, increasing the separation $\Delta$ strengthens it relative to OLS\textsubscript{pooled}.
\hemant{This discussion seems to be for synthetic experiments, not real data?}

\subsection{Additional Plots}
  \begin{figure}[H]
    \centering
    \includegraphics[width=\linewidth]{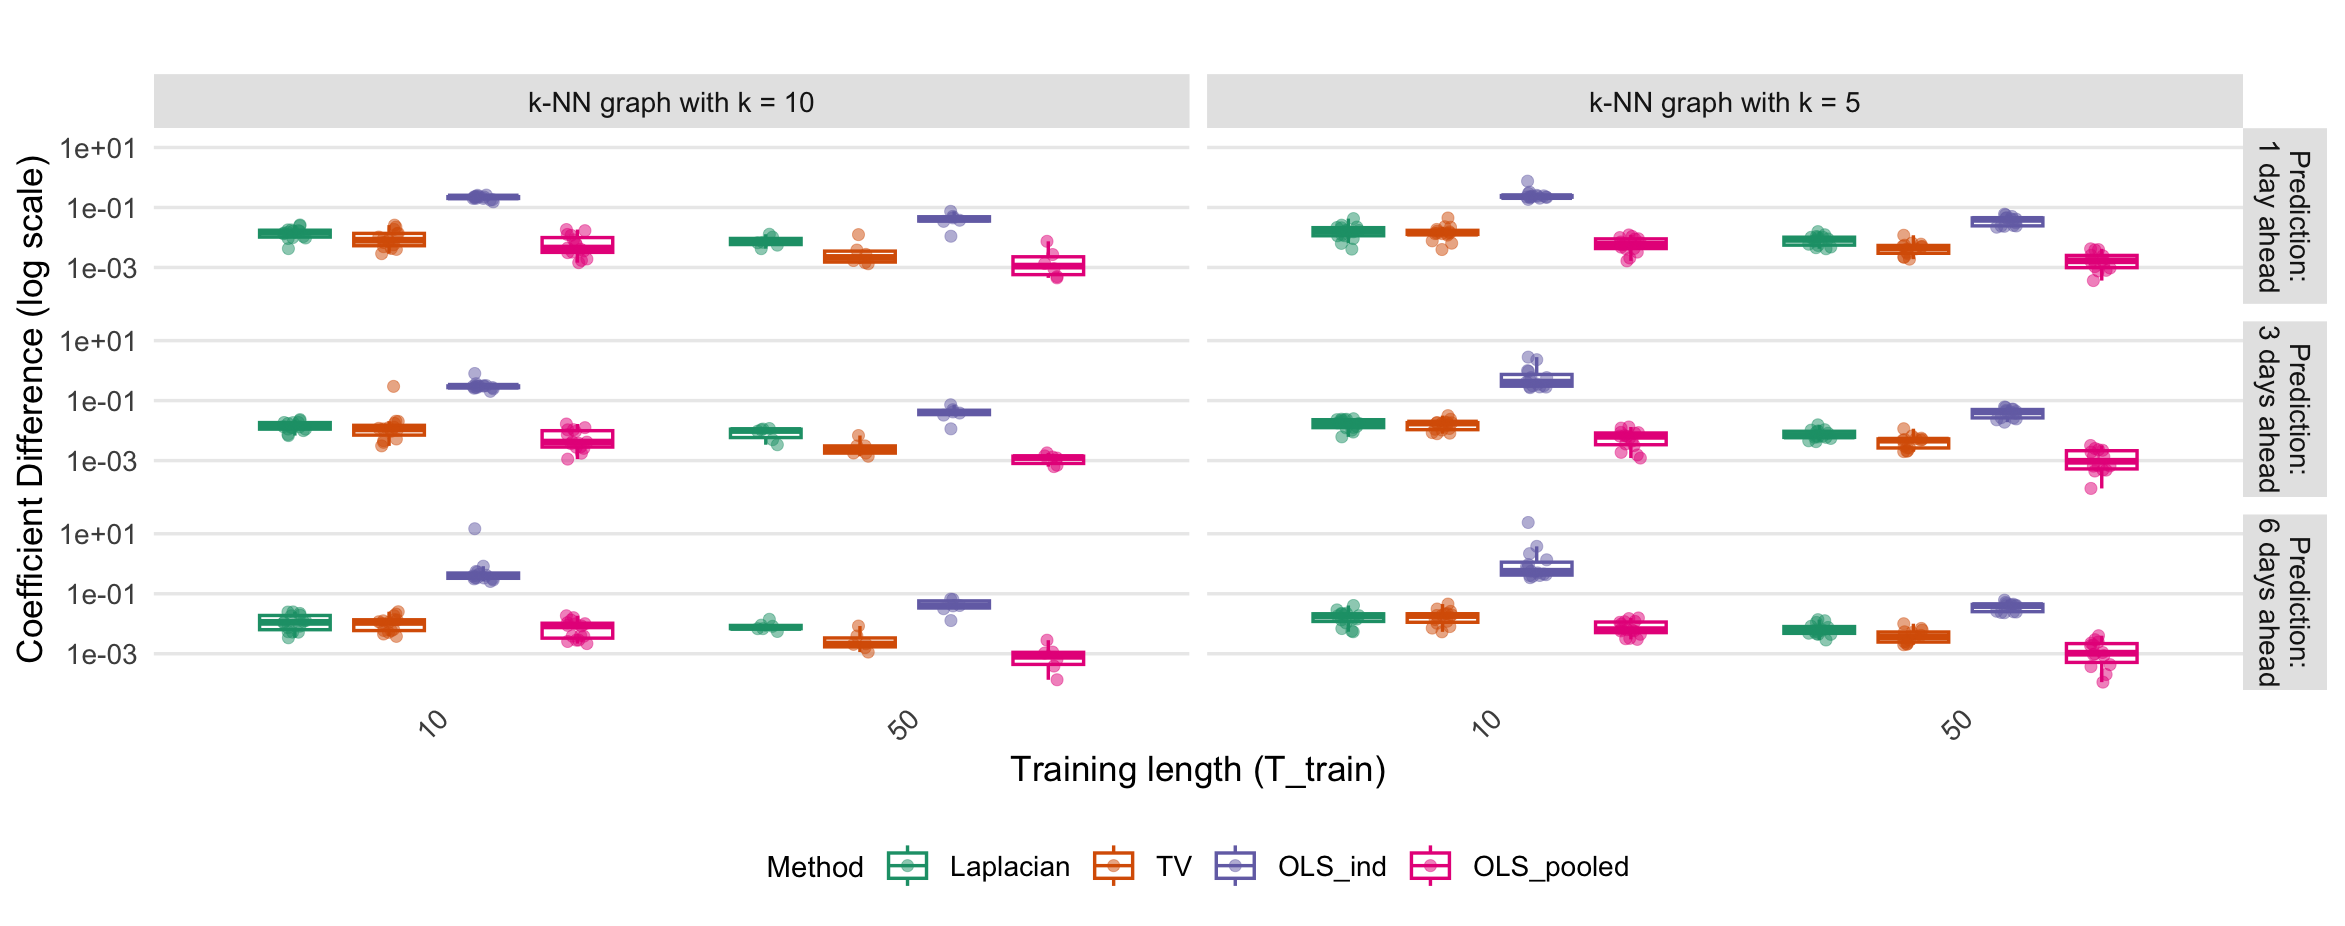}
  \caption{Coefficient stability for the NO dataset. We vary the training length ($T_{\text{train}} \in \{10, 50\}$), as well as the number of neighbours used to construct the graph ($k$). Boxplots show the distribution of errors over 15 independent trials (years). }
  \label{fig:results_all_no}
  \end{figure}

  \begin{figure}[H]
    \centering
    \includegraphics[width=\linewidth]{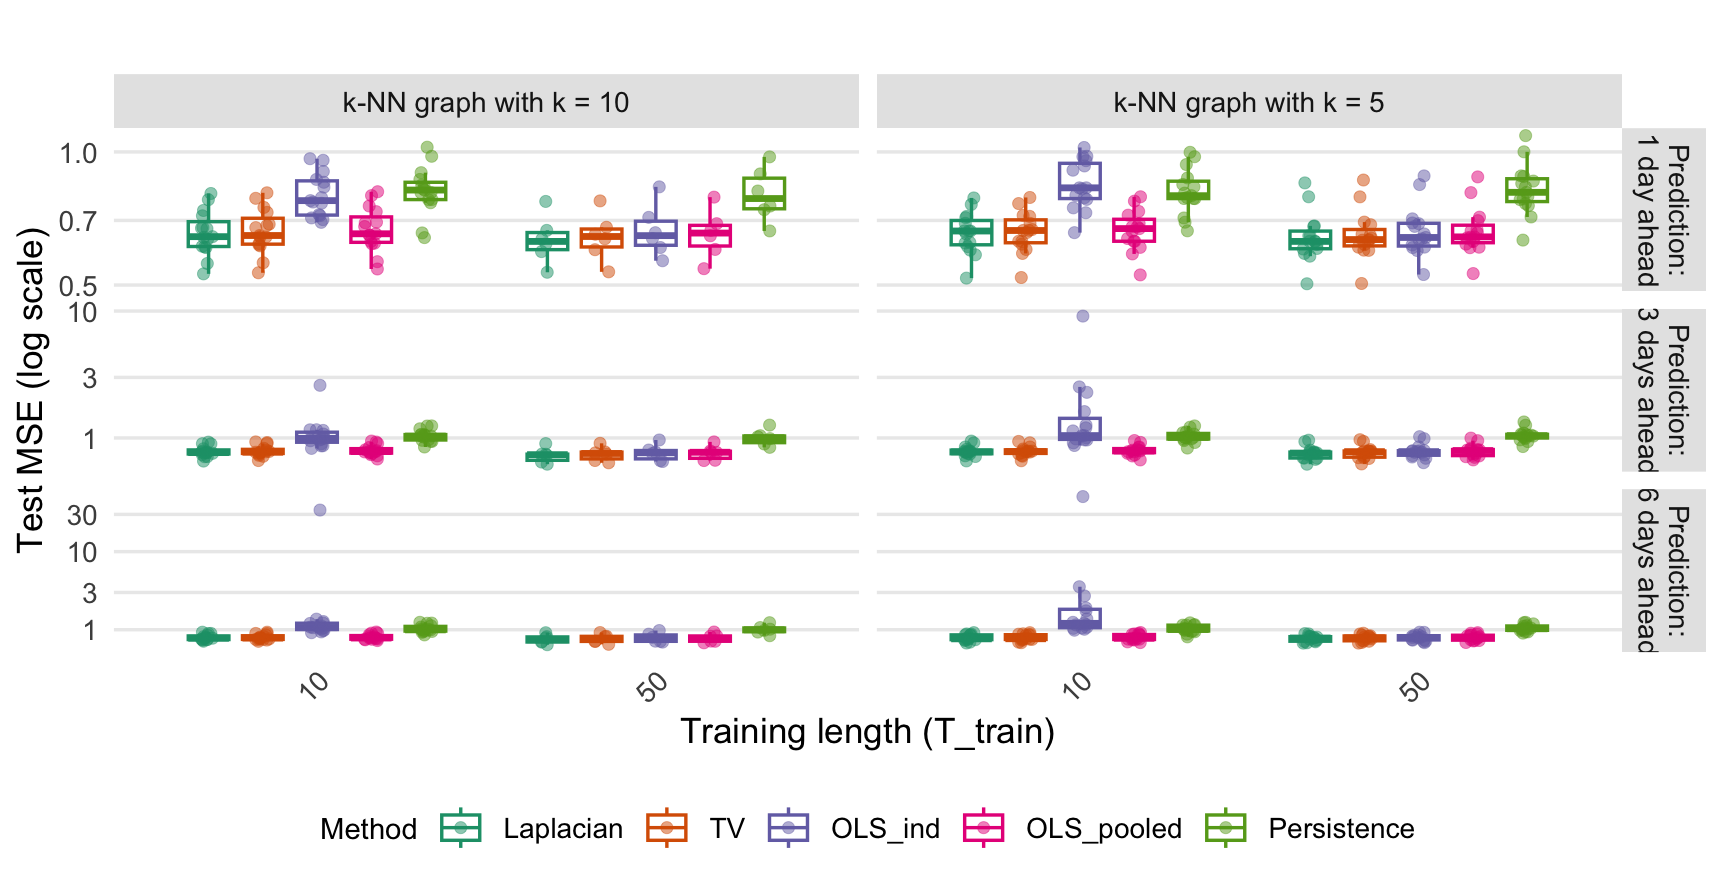}
  \caption{ Test RMSE for predicting pollutant concentration on the next day for the NO  dataset. We vary the training length ($T_{\text{train}} \in \{10, 50\}$), as well as the number of neighbours used to construct the graph ($k$). Boxplots show the distribution of errors over 15 independent trials (years). }
  \label{fig:results_no_test_all}
  \end{figure}

  \begin{figure}[H]
    \centering
    \includegraphics[width=0.8\linewidth]{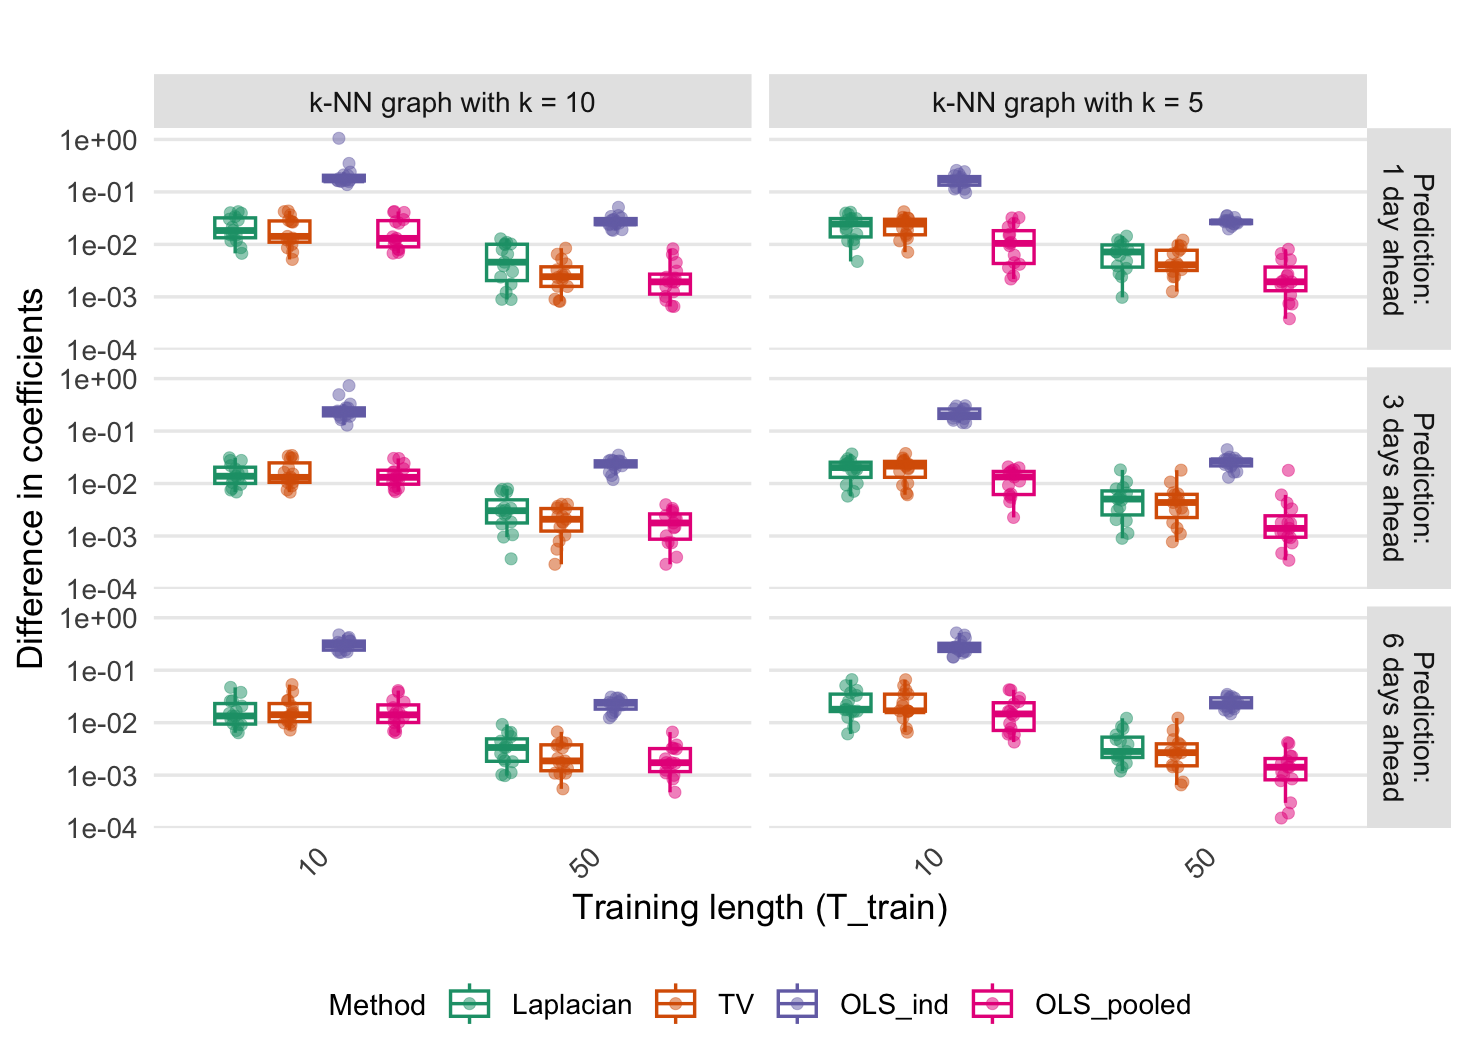}
      \caption{Coefficient stability for predicting pollutant concentration on the next day for the  PM10 dataset. We vary the training length ($T_{\text{train}} \in \{10, 50\}$), as well as the number of neighbours used to construct the graph ($k$). Boxplots show the distribution of errors over 15 independent trials (years). }
  \label{fig:results_pm10_sta}
  \end{figure}

  \begin{figure}[H]
    \centering
    \includegraphics[width=0.8\linewidth]{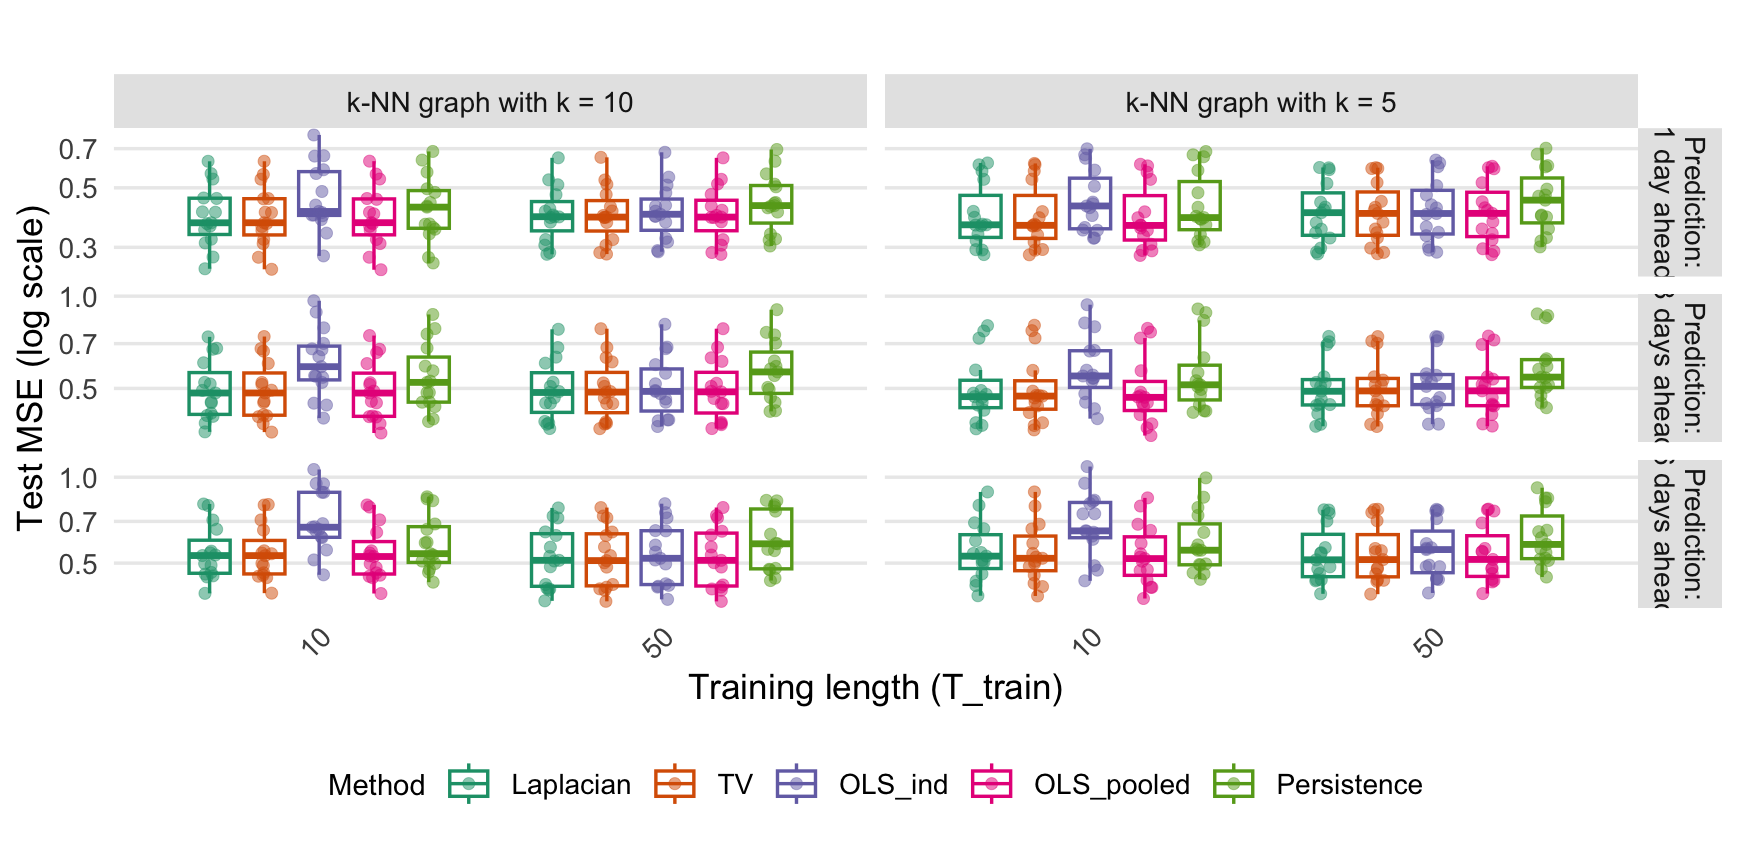}
  \caption{ Test RMSE for predicting pollutant concentration on the next day for the PM10 dataset. We vary the training length ($T_{\text{train}} \in \{10, 50\}$), as well as the number of neighbours used to construct the graph ($k$). Boxplots show the distribution of errors over 15 independent trials (years). }
  \label{fig:results_pm10_test}
  \end{figure}
